# Supplementary material for: In-Context Brush: Zero-shot Customized Subject Insertion with Context-Aware Latent Space Manipulation
Source: arXiv:2505.20271 source file (2025-05-26)
Supplement: Supplementary file 1 [file supp1.tex]

\begin{figure*}[h]
  \centering
  \includegraphics[width=0.85\linewidth]{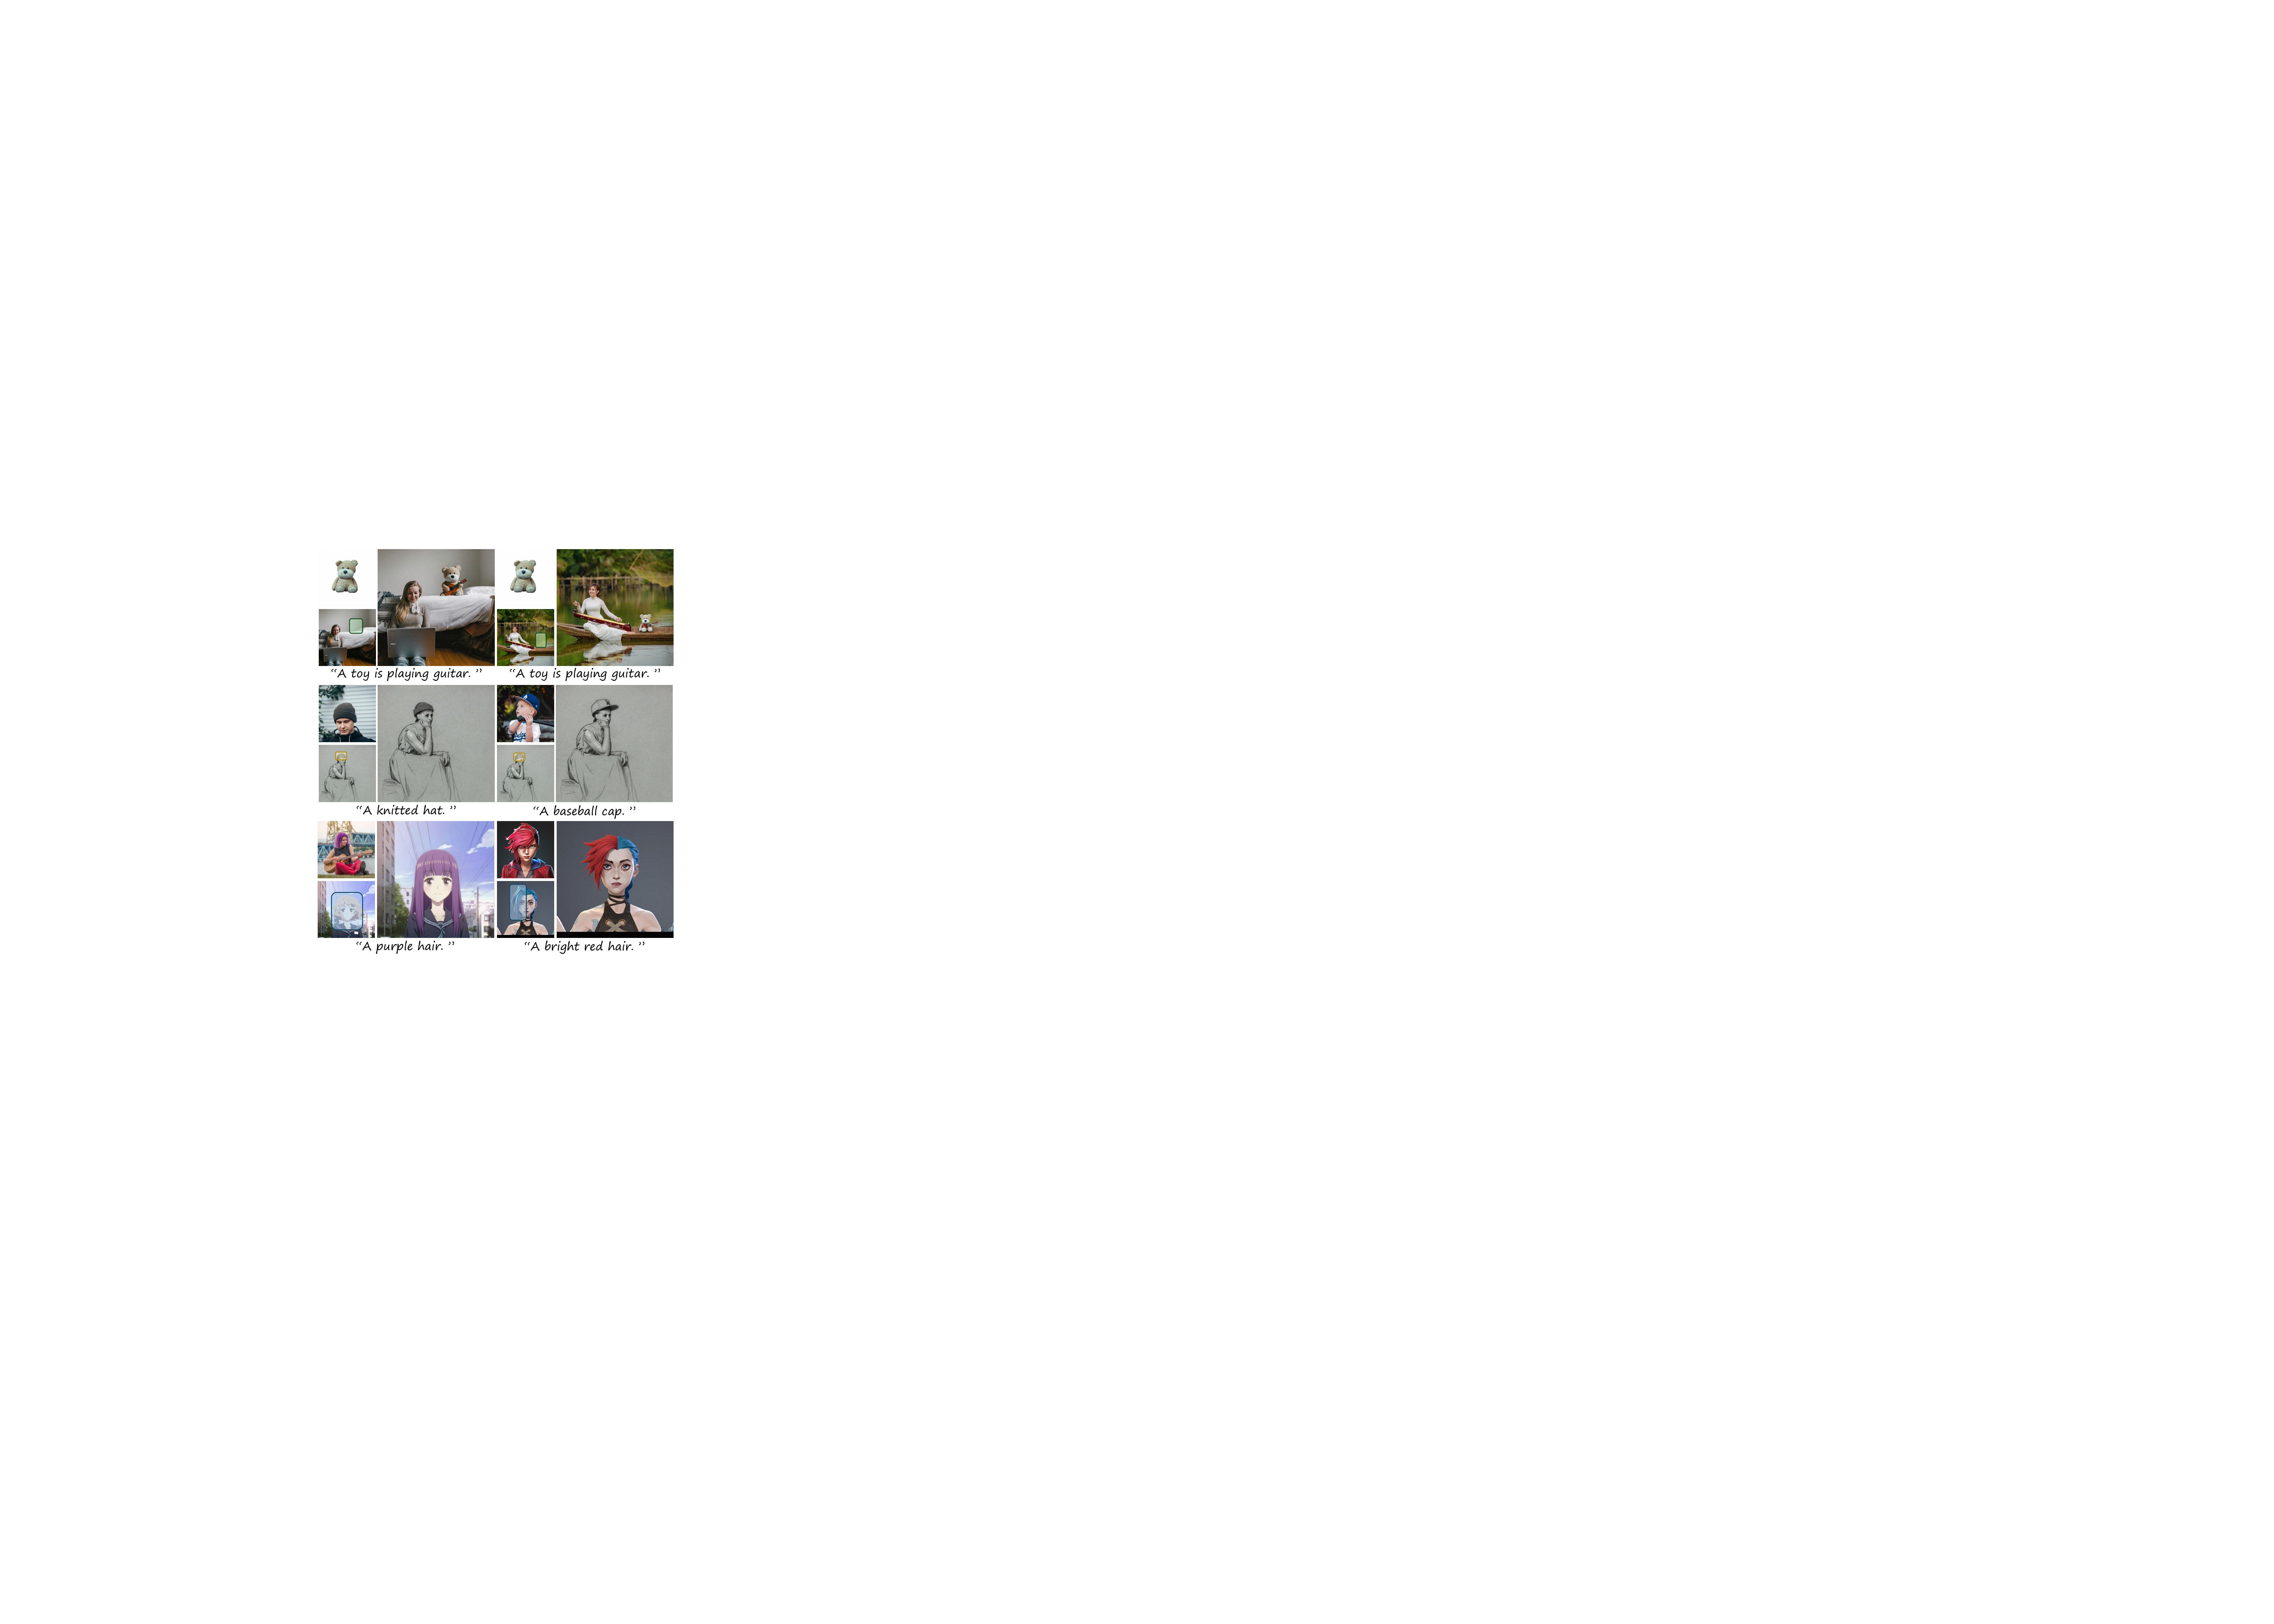}
  \caption{\textbf{Additional results of our method.}}
  \label{fig:supp1}
\end{figure*}
